# Supplementary material for: Updated Standard for Secure Satellite Communications: Analysis of Satellites, Attack Vectors, Existing Standards, and Enterprise and Security Architectures
Source: arXiv:2310.19105 source file (2023-10-29)
Supplement: Supplementary file 1 [file AppendixTemplate.tex]

% Appendix Template

\chapter{Appendix Title Here} % Main appendix title

\label{AppendixX} % Change X to a consecutive letter; for referencing this appendix elsewhere, use \ref{AppendixX}

Write your Appendix content here.
